# Supplementary material for: Ultracompact programmable silicon photonics using layers of low-loss phase-change material Sb$_2$Se$_3$ of increasing thickness
Source: arXiv:2409.12582 ancillary file (2024-09-19)
Supplement: Supplementary file 1 [file Blundell2024_SI.pdf]

# Supporting Information: Ultracompact programmable silicon photonics using layers of low-loss phase-change material $Sb_2Se_3$ of increasing thickness.

Sophie Blundell,[†,‡] Thomas Radford,[‡] Idris A. Ajia,[‡] Daniel Lawson,[‡] Xingzhao Yan,[†] Mehdi Banakar,[†] David J. Thomson,[†] Ioannis Zeimpekis,[†,¶] and Otto L. Muskens[*,‡]

†*Optoelectronics Research Centre, University of Southampton, Southampton, UK*

‡*School of Physics and Astronomy, University of Southampton, Southampton, UK*

¶*Electronics and Computer Science, University of Southampton, Southampton, UK*

E-mail: o.muskens@soton.ac.uk

Phone: +44 (0)23 80593911

## 1 Simulation

Computational modelling of PICs is a useful tool for designing PICs as well as confirming experimental results. Modelling the propagation of beams through waveguiding structures is a non-trivial problem due to the complexity of calculating propagating modes and due to the need to impose boundary conditions upon time-dependent Maxwell's equations. This could be addressed using the finite-difference beam propagation method (BPM) as set out by Xu and Huang in 1995,[1] but this BPM approach relies on a slowly-varying envelope

approximation which may not be appropriate for discontinuous media or high-index contrast materials, both of which apply to including a PCM in a waveguide structure. Instead, a finite-difference time-domain (FDTD) approach can be taken, as first introduced by Yee in 1966.[2] The time-domain aspect of FDTD allows multiple frequency analysis, enabling a broadband response to be calculated, as well as providing more intuitively understandable simulations. An extra benefit of using FDTD is that the mesh structure used over the physical structure does not have to be uniform, so can more realistically model a PIC. FDTD involves discretising the overall structure into "cells", and solving Maxwell's equations for each cell in turn in the direction of propagation. The main downside of using an FDTD approach is that the size of device that can be modelled is limited by the computational resources available. Such simulation can be made more efficient, and more practically possible for larger devices, by using a 2D simulation as opposed to a full 3D simulation. Where light is propagating solely in-plane within a PIC and assuming that there is minimal coupling between modes, the effective refractive index method can be employed, which uses the effective index of the first cell, calculated by collapsing the 3D geometry, to calculate the effective index for the next cell, again in the direction of propagation.[3] Using this method is a way to simulate a 3D structure by considering only 2D propagation which essentially reduces the dimensionality of the problem and is sometimes called 2.5D variational FDTD as it offers comparable accuracy to a 3D simulation with a similar run time to a 2D simulation.

The Lumerical MODE variational FDTD software package was used to simulate the silicon photonic waveguides in this work. The structure shown in Fig. 1 was constructed, featuring an $Sb_2Se_3$ block. This waveguide cross-section has a 3 $\mu$m thick $SiO_2$ substrate, 100 nm thick silicon layer and 220 nm thick silicon rib waveguide. For the purpose of simulating a waveguide with this cross-sectional geometry, in three dimensions the model waveguide has a length of 200 $\mu$m, with the $Sb_2Se_3$ block spanning the centre 50 $\mu$m of this. An X-normal eigenmode solver is added to the simulation, centred on the rib waveguide and $Sb_2Se_3$ block, with a size of $2 \times 1$ $\mu m^2$ in the y and z dimensions respectively. With $Sb_2Se_3$ layered on top

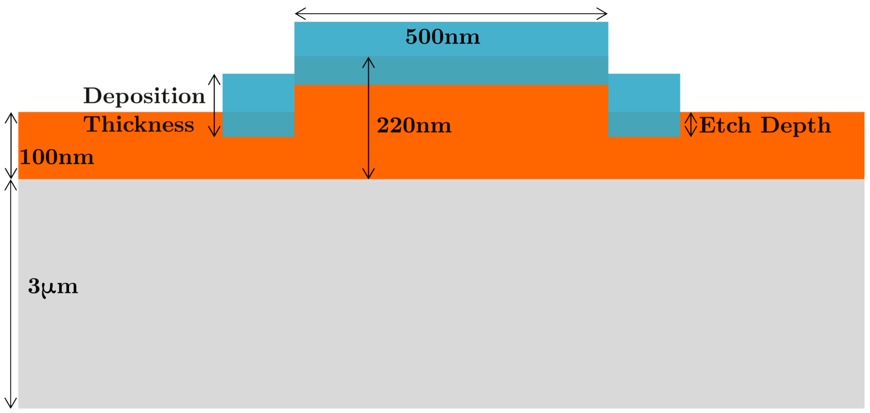


Figure 1: The structure simulated for a variety of deposition thicknesses and etch depths of $Sb_2Se_3$ , featuring a silicon rib waveguide and silica substrate.

of the waveguide thickness values of $Sb_2Se_3$ between 20 nm and 100 nm were simulated. A source of light, injected in the positive x-direction at 10 $\mu$m from the end of the waveguide and with a wavelength of 1550 nm allows measurement of the change in transmission of this light when the $Sb_2Se_3$ block is altered.

As a measure of the difference in refractive index profile of the structure, $n_{\text{eff}}$of fundamental mode of the light injected is plotted for $Sb_2Se_3$ in both its crystalline and amorphous phases in Fig. 2 for the six values of $Sb_2Se_3$ layer thickness on the surface of the waveguide. It can be seen that for thicker layers the difference in $n_{\text{eff}}$increases, meaning that a larger change in transmission for switching the material's state can be achieved with a thicker layer. While $n_{\text{eff}}$increases with thickness of $Sb_2Se_3$ , there is a limit to this trend beyond a thickness of 60 nm. This limit is attributed to the way that the light is interacting with the $Sb_2Se_3$ , via evanescent coupling, which normally sees amplitude of light rapidly decay with distance.

## 1.1 Etched Waveguides for Enhanced Modulation

Before the PCM deposition process it is possible to etch into the surface of a silicon waveguide. In doing so, prior to deposition of $Sb_2Se_3$ , the PCM can effectively replace part of the silicon waveguide, making the mode overlap larger and thus the change in transmission enacted by switching the $Sb_2Se_3$ larger. This effect can be simulated using Lumerical

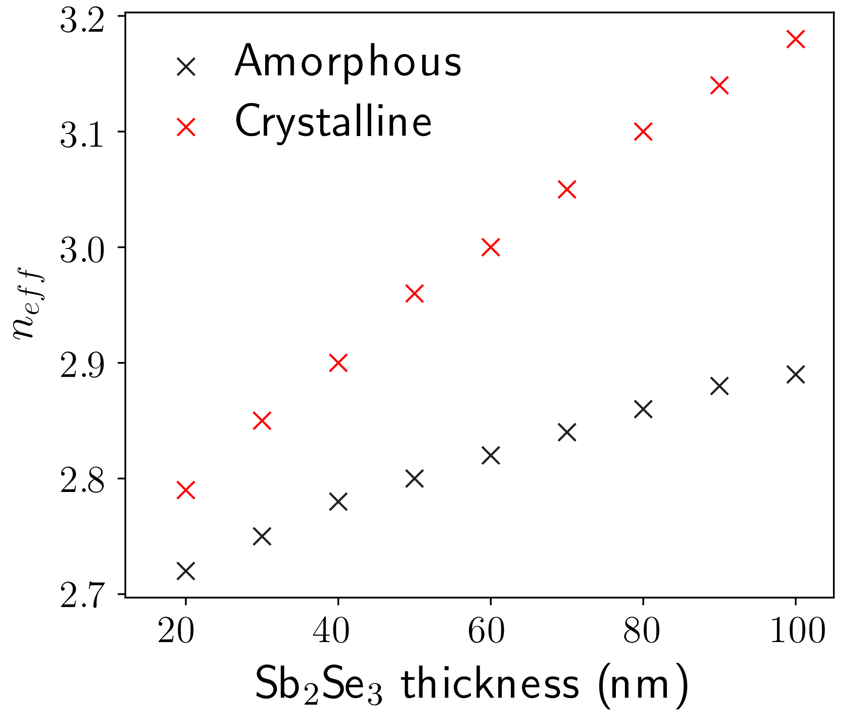


Figure 2: Effective refractive index of fundamental modes for different thicknesses of $Sb_2Se_3$ deposited on the surface of a silicon waveguide in the crystalline and amorphous states.

FDTD by changing the structure of the waveguide model. In this case, an eigenmode solver is used, centred again on the waveguide and $Sb_2Se_3$ block, and the $n_{\text{eff}}$of the fundamental mode recorded for etch depths and deposition thicknesses between 0 and 100 nm. Investigating the parameter space for etch depth and deposition thickness shows, in Fig. 3, that the highest change in effective refractive index occurs for the 100 nm deposition with an etch depth of 100 nm. The dashed line in this Figure indicates the design conditions used for the MMI optimization. Experimentally, the etch depth does not reach this condition, as indicated by the SEM cross-sections. The other limiting case of zero etching is indicated by the dash-dotted line in Fig. 3. The corresponding values for these two limiting cases are plotted in Fig. 4, corresponding to the cross sections of the map of Fig. 3. We see a similar trend in $\Delta n_{\text{eff}}$ against thickness of $Sb_2Se_3$ for etched and unetched waveguides, indicating a that etch depth mainly affects the absolute value of the switching. Quantitatively, the difference in $\Delta n_{\text{eff}}$ between the fully etched and zero etched conditions is equivalent to an

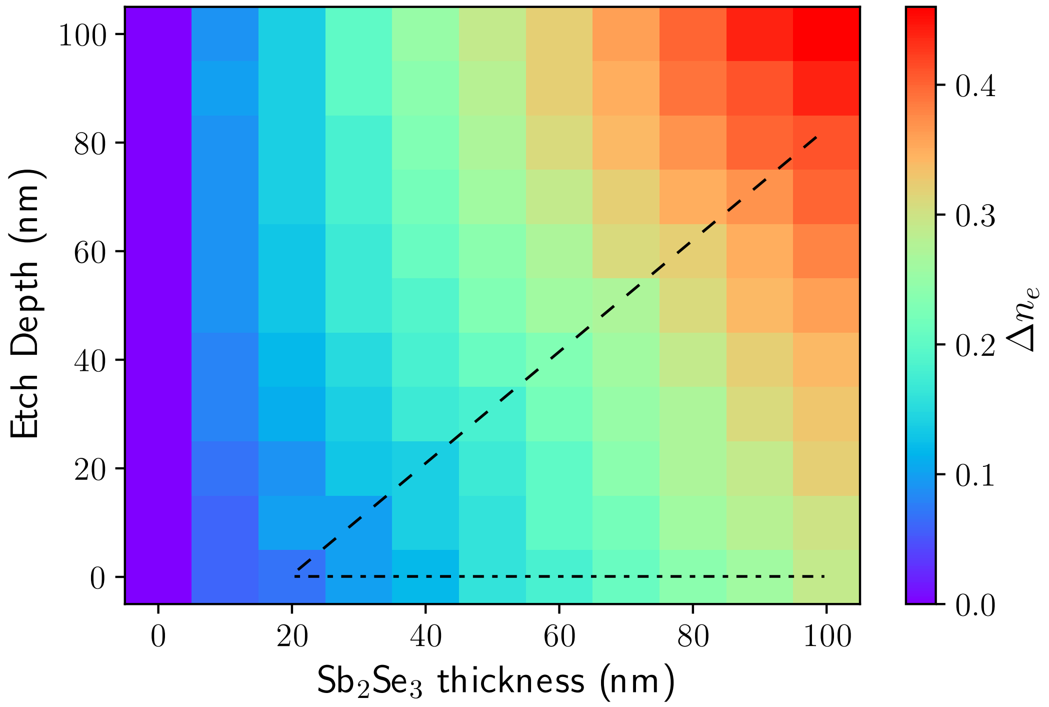


Figure 3: Change in effective refractive index between the crystalline and amorphous states of a waveguide embedded with $Sb_2Se_3$ when the material thickness and depth of the etch performed prior to $Sb_2Se_3$ deposition are varied. Dashed line: design used for MMI optimization; dash dotted line: no etch.

variation in the $Sb_2Se_3$ layer thickness of up to 20 nm for the thickest layers in this study.

## 1.2 Silicon Chip Fabrication

The chips used in this project were fabricated using Deep-UV projection lithography, where a UV beam is scanned directly over the photolithography mask, projecting the chip design onto a wafer. Deep-UV lithography is typically used in industry due to its rapidity, scalability and production ready capabilities, but other lithography tools such as electron-beam lithography are frequently used in research where greater versatility of feature size is required. Rib waveguides were formed by etching 120 nm into the surface layer of silicon with a 2 $\mu$m wide trench region. Grating couplers were written with an etch depth of 70 nm and width of 1 $\mu$m, tapering down to a 500 nm width waveguide for single mode propagation. All

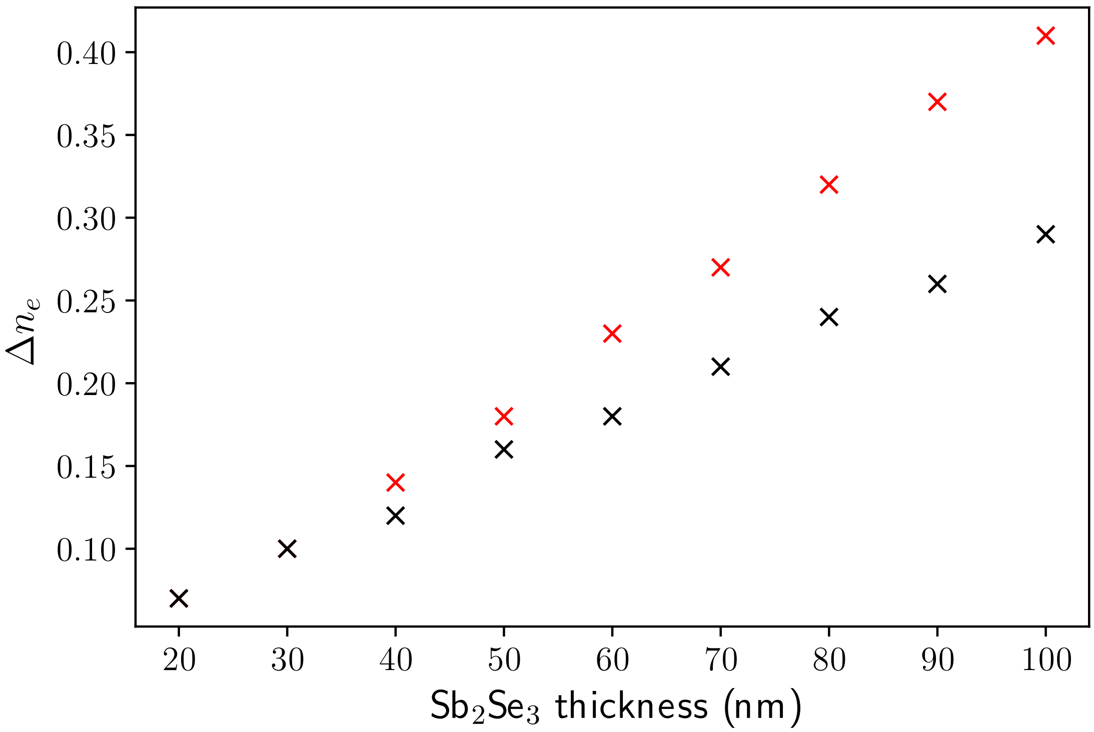


Figure 4: Cross-sections of Figure 3 showing induced change in effective refractive index $n_{\text{eff}}$ of the fundamental mode when $Sb_2Se_3$ is switched from the amorphous to the crystalline states against $Sb_2Se_3$ thickness, when the material is deposited on the surface of the waveguide (black crosses) and when the waveguide is partially etched (red crosses).

chips contain a variety of waveguide devices, and are left with an open window following a second DUV exposure with alignment of the deposition windows to the waveguides ready for etching and deposition of $Sb_2Se_3$ .

# 2 Setup

## 2.1 Spectral Analysis

The experimental setup used was a conventional silicon photonics spectral analysis setup. The setup used for this experiment employed an Agilent Technologies tunable laser source with built-in detector. This light is coupled into the chip under test through the grating couplers at the inputs and outputs of a device and coupled out again to the detector via

optical fibres, mounted on fixed-angle fibre arms. The chip is placed on a stage which is capable of motion in all three dimensions and viewed through a digital camera from above for fibre alignment.

In order to investigate the difference in spectral insertion loss through a variety of devices incorporating $Sb_2Se_3$ at a thickness of 80 nm and etch depth of 60 nm when the PCM is switched, an as-deposited amorphous sample was first tested. For every device on the chip, an insertion loss spectrum from 1520 - 1570 nm was taken, both for devices with $Sb_2Se_3$ embedded as well as those without for the purpose of referencing. The chip was then annealed at 190°C for 10 minutes in order to crystallize the $Sb_2Se_3$ areas within the devices. Then, the spectral loss measurements were repeated.

## 2.2 In-situ Optical Spectroscopy and Laser Writing of Phase Change Components

This experimental setup is capable of both optically switching the material and measuring C-band telecommunication wavelength transmission through the waveguides. This was used to demonstrate the switching capabilities of the novel method used in this project to embed $Sb_2Se_3$ into silicon photonic waveguides. Switching was performed using a Vortran 638 nm laser, digitally gated using a Berkeley Nucleonics programmable pulse generator, with light directed onto the surface of the sample via a Mitutoyo 50× objective, with NA 0.65 and focal length 4 mm. Gating the pulse using a pulse generator allows control of the pulse down to nanosecond lengths and utilising the full 170 mW power capability of the laser in increments, enabling production of the required pulses for PCM switching. Light is coupled into the device via optical fibres from a tunable laser source to a detector, hence changes in transmission due to phase change of the material can be measured as change in transmission through the device.

To isolate the effect of changing the phase of $Sb_2Se_3$ integrated into a photonic waveguide, MZIs were measured. Measuring an MZI allows extraction of the phase shift from

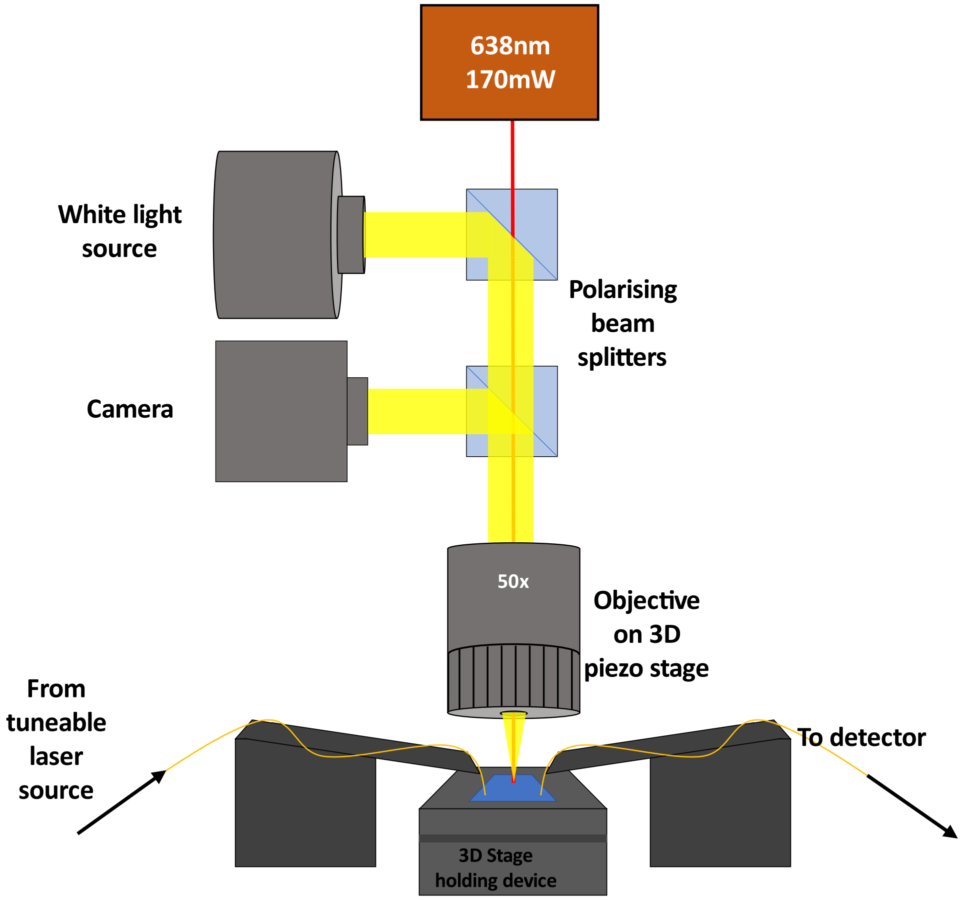


Figure 5: Optical setup used for simultaneous fibre-coupled spectroscopy and direct-write optical switching of PCMs from the top of the device under test.

interference spectrum which is robust to variations in the coupling efficiency, for example, due to environmental fluctuations. Measuring through an interferometer provides direct self-referencing as the light travels through two waveguide arms, one clad in $Sb_2Se_3$ , so that the resulting interference pattern provides a measure of the phase shift incurred through one arm compared to the unclad arm.

Initially, MZIs were measured for the five different deposition thicknesses fabricated, for the six available lengths of crystalline PCM deposited on the top arm of each MZI, to investigate the losses incurred at each. Then, for a PCM length of 50µm, as-deposited amorphous $Sb_2Se_3$ was crystallized 1 $\mu$m at a time, with the spectrum measured after each switching event, showing the gradual phase shift possible by increasing the amount of crystalline material included in one arm. Switching between the two states was then

demonstrated, beginning in an as-deposited amorphous state, crystallising 1 $\mu$m at a time and then amorphising 1 $\mu$m at a time to return to the initial state.

This experimental setup was controlled by a labVIEW program written in order to pattern the material and measure transmission through a double fibre output arm simultaneously. During the experiment a pixel pattern was written on an MMI to change the ratio of the output couplers, thus demonstrating use of $Sb_2Se_3$ for programmability. Each pattern was trialled in the setup, crystallizing pixels on an amorphous background and measuring the transmission through both output couplers after each pixel is crystallized. From these measurements, the change in the splitting ratio between the two output couplers can be observed.

This was then performed with a crystalline background and amorphous pixels written. Initially, an amorphous background was chosen as the refractive index of amorphous $Sb_2Se_3$ is closer to that of silicon than its crystalline refractive index, meaning that loss is minimized in the amorphous state. However, in practice, writing crystalline spots onto an amorphous background is less easy to control than writing amorphous spots onto a crystalline background, in part due to their larger size, and also the nature of crystals to grow when close to other crystals.

# 3 Fitting

Experimental results for insertion loss measurements on the MZIs were fitted using a nonlinear least-squares method implemented in Python through the lmfit package.

First, spectra were converted from wavelength to frequency scale and resampled to equal frequency steps, in order to facilitate fitting using a periodic frequency comb function. To provide an initial value for fitting, the free-spectral range (FSR) of the first spectrum (before laser writing) was extracted by using a fast-fourier transform. The first spectrum was subsequently fitted to the MZI response function, resulting in values for the transmission,

contrast and FSR.

For subsequent spectra, the starting value of the first FSR was used as an input for the next spectrum, where the fitting was constrained to a small variation of less than 0.1% of this frequency to take into account the shifting of the peak. The fitted FSR for each spectrum was then used as a starting point of the next spectrum in the series. This method allowed the fits to converge well even for low contrast values. Typical results are shown in 6a for the device with 20 nm $Sb_2Se_3$ thickness, where the red curves indicate the fits and black curves the experimental spectra. Resulting values for the transmission, contrast and FSR are given in 6b.

To complement the subset of results shown in the main text, full sets of data are presented in Fig. 7 for the five MZI devices for different $Sb_2Se_3$ thickness. We also performed measurements on two other chips with similar devices, yielding very similar results, results are shown in Fig. 8 and Fig. 9. In these two chips, a thin $SiO_2$ buffer layer was deposited between the Si waveguide and the PCM. The similarity of results indicate that the oxide buffer layer has no measurable effect on the performance of the hybrid PCM-Si photonics device.

In the presentation of our main results in Fig. 3 of the main text, we have chosen to show wavelength shift at a selected wavelength to illustrate the effect of the switching of the PCM on the spectral response. The wavelength shift was then used in combination with the FSR wavelength in this part of the spectrum, to extract the phase shift $\Delta\phi$.

In a more formal analysis one can express the frequency shift $\Delta f$ in terms of the change of the FSR frequency itself, $\Delta f_{FSR}$, times the mode number $N$, $\Delta f = N\Delta f_{FSR}$. For the example in Fig. 6, the mode at frequency 196.6 THz corresponds to $N = 475$ given the FSR of $f_{FSR} = 0.41385$ THz. In Fig. 10 we plot the normalized $f_{FSR}$ against length of the switched PCM for the different $Sb_2Se_3$ thickness. We see a change in FSR over the switched device length of up to 1.2% for the 80 nm thick $Sb_2Se_3$ layer, compared to a change of around 0.1% for the 20 nm $Sb_2Se_3$ layer. The phase shift per unit length $\Delta\phi$ then follows as

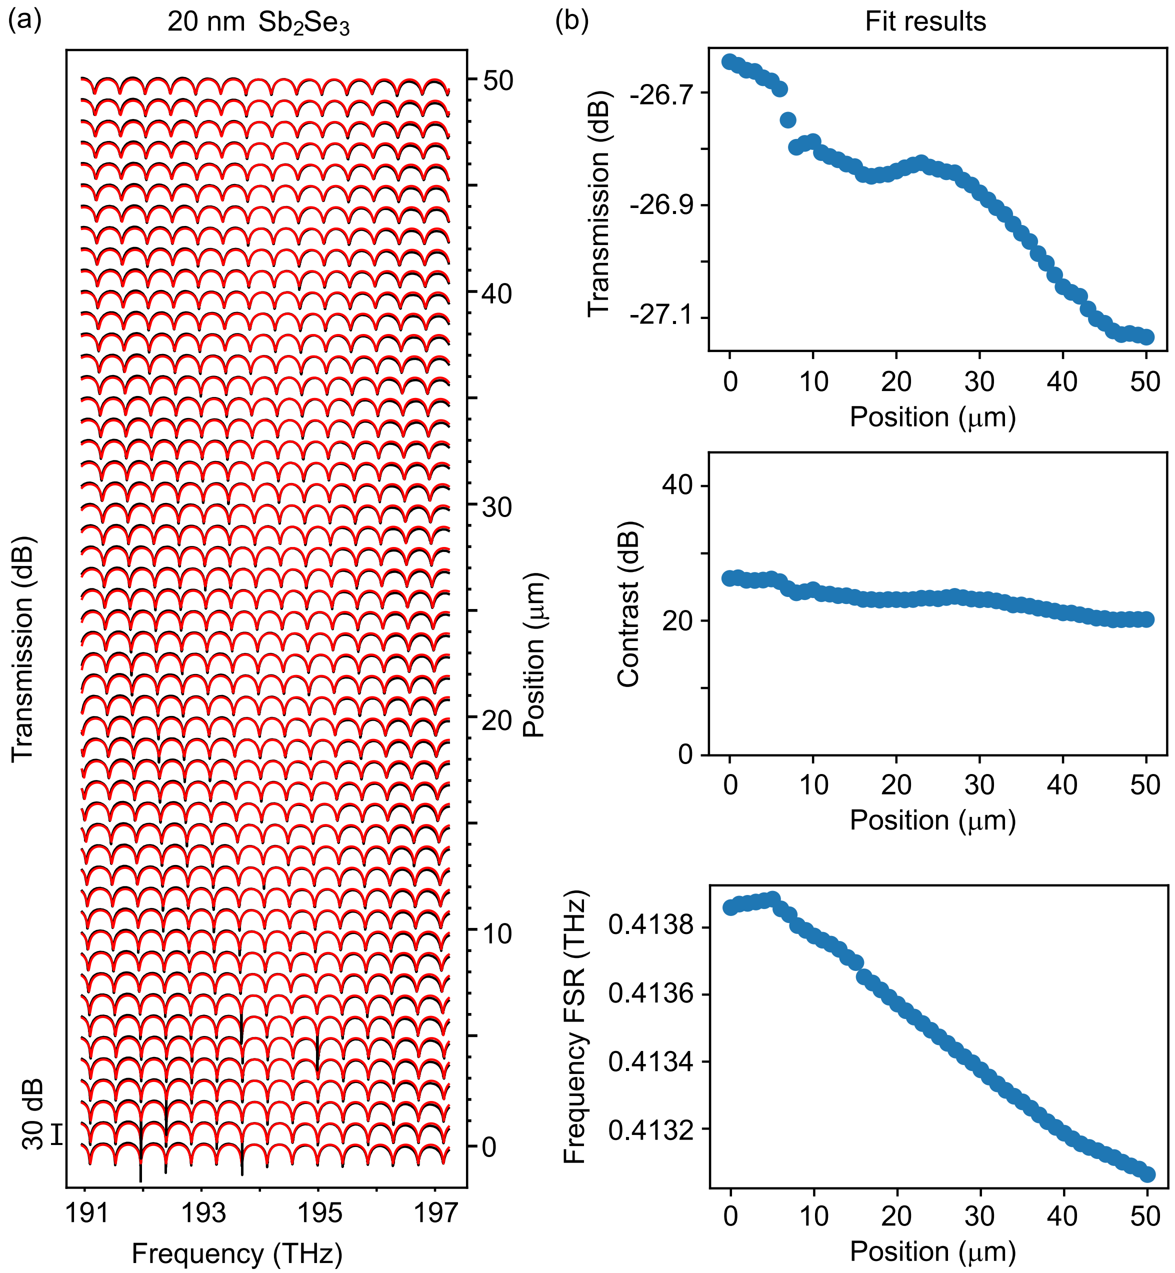


Figure 6: **Example of fitting MZI transmission spectra for 20 nm $Sb_2Se_3$ .** (a) All spectra corresponding to map of Fig. **??** (Fig. 2a in main text), for experimental data (black curves) and model fits (red curves). (b) Fitting results for absolute transmission, MZI extinction contrast and free spectral range (c), against position of the write laser on the PCM slab.

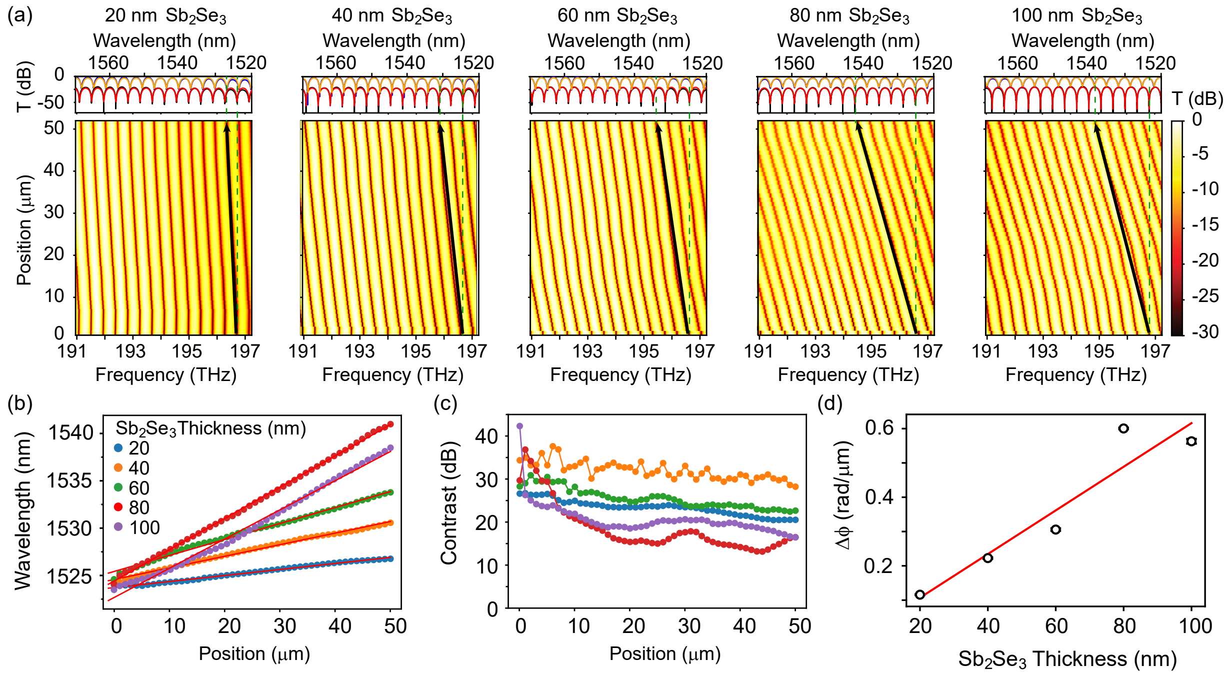


Figure 7: **Results on chip without oxide buffer layer.** (a) Spectra of MZIs before and after crystallization (top panels) and maps taken after every $1\mu$m of crystallization (bottom panels) by direct laser writing over $50\mu$m of $Sb_2Se_3$ , for devices with $Sb_2Se_3$ thickness of 20, 40, 60, 80, 100 nm. Black/blue curves in top panel: experimental spectra, red/orange curves: model fits. Vertical dashed lines indicate shift of selected mode with initial wavelength around 1524 nm. (b, c) Wavelength position (b) and contrast (c) extracted from fits to experimental spectra for MZI devices with $Sb_2Se_3$ thickness between 20 nm and 100 nm. Red lines: linear fits to data. (d) Extracted values of slope $\Delta\phi$ plotted against $Sb_2Se_3$ thickness. Red line: linear fit.

$\Delta\phi = 2\pi\Delta f_{\mathrm{FSR}}/L$ resulting again in Fig. 7d or the corresponding Fig. 3d in the main text.

# 4 Reversibility of switching

To investigate the reversibility of the switching, we measured spectra of the laser-crystallized MZI by re-amorphizing and re-crystallizing the same device. Amorphization of the same areas of $Sb_2Se_3$ was done for devices with $Sb_2Se_3$ thickness of 40 nm, 60 nm and 80 nm. Spectra were taken after each switching event, totally 125 spectra for each deposition, as the amorphization spot was approximately two thirds the size of the crystallising spot, giving 75 switching events for amorphizing and 50 for crystallising. The spectra are shown in Fig.

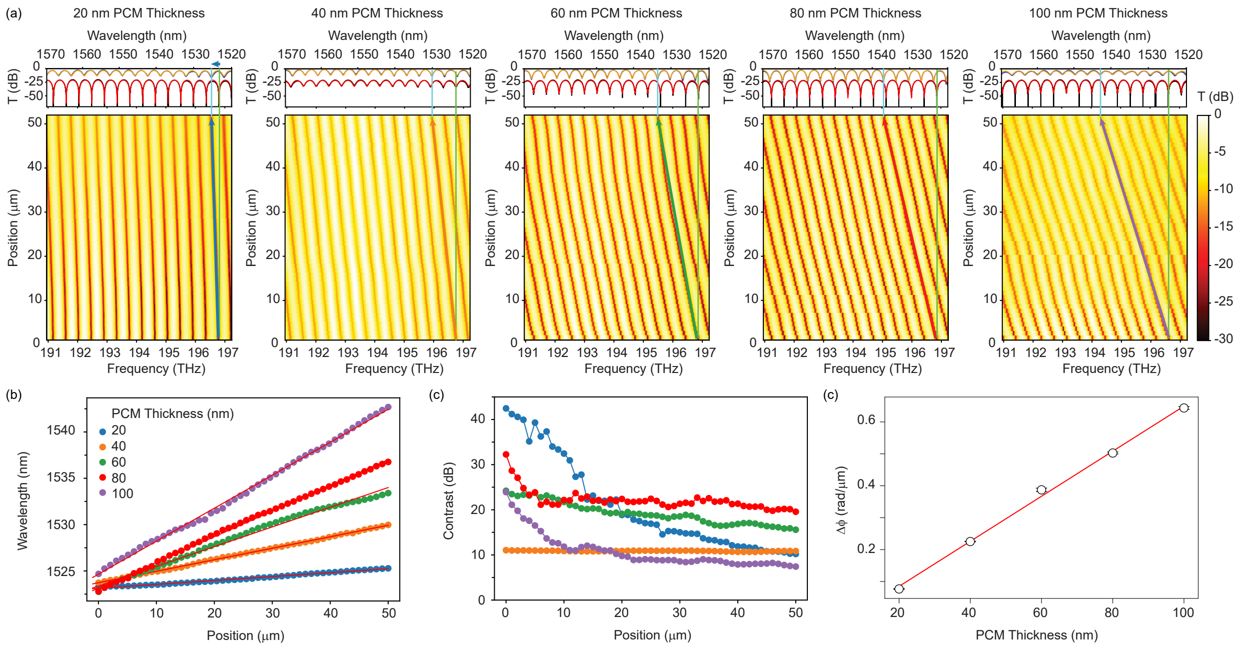


Figure 8: **Results on chip with oxide buffer layer, set 1.** (a) Spectra of MZIs before and after crystallization (top panels) and maps taken after every 1$\mu$m of crystallization (bottom panels) by direct laser writing over 50$\mu$m of $Sb_2Se_3$ , for devices with $Sb_2Se_3$ thickness of 20, 40, 60, 80, 100 nm. Black/blue curves in top panel: experimental spectra, red/orange curves: model fits. Vertical dashed lines indicate shift of selected mode with initial wavelength around 1524 nm. (b, c) Wavelength position (b) and contrast (c) extracted from fits to experimental spectra for MZI devices with $Sb_2Se_3$ thickness between 20 nm and 100 nm. Red lines: linear fits to data. (d) Extracted values of slope $\Delta\phi$ plotted against $Sb_2Se_3$ thickness. Red line: linear fit.

11, from which the wavelength shift was extracted to give Fig. 12. As the pre-crystallized material is gradually amorphized, the wavelength of a selected spectral peak shifts in the negative direction, and as it is gradually recrystallized, this peak shifts back in the positive direction, returning to its initial position, with an accuracy ranging from 3-20% of the initial value.

# 5 Results for switching of 60 nm $Sb_2Se_3$

In order to reduce the density of results in the main text, a subset of results were presented in Figs. 4 and 5 for $Sb_2Se_3$ thickness of 20, 40, 80, and 100 nm. Figure 13 summarizes

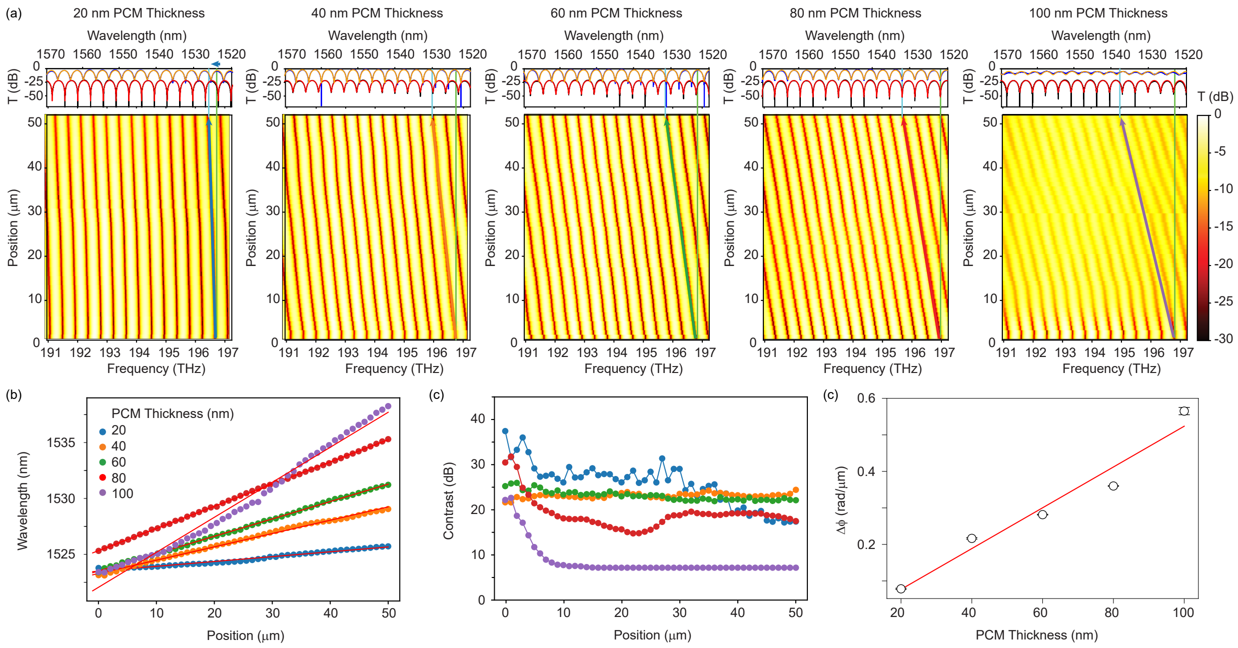


Figure 9: **Results on chip with oxide buffer layer, set 2.** (a) Spectra of MZIs before and after crystallization (top panels) and maps taken after every 1$\mu$m of crystallization (bottom panels) by direct laser writing over 50$\mu$m of $Sb_2Se_3$ , for devices with $Sb_2Se_3$ thickness of 20, 40, 60, 80, 100 nm. Black/blue curves in top panel: experimental spectra, red/orange curves: model fits. Vertical dashed lines indicate shift of selected mode with initial wavelength around 1524 nm. (b, c) Wavelength position (b) and contrast (c) extracted from fits to experimental spectra for MZI devices with $Sb_2Se_3$ thickness between 20 nm and 100 nm. Red lines: linear fits to data. (d) Extracted values of slope $\Delta\phi$ plotted against $Sb_2Se_3$ thickness. Red line: linear fit.

the corresponding results for the 60 nm $Sb_2Se_3$ , both for amorphous pixels on crystalline background (top panel) and crystalline pixels on amorphous background (bottom panel). These findings are in line with the other results and lie in between those of the 40 nm and 80 nm thick $Sb_2Se_3$ layers in terms of number of pixels.

# References

(1) Xu, C. L.; Huang, W. P. Finite-Difference Beam Propagation Method for Guide-Wave optics. *Progress in Electromagnetics Research* **1995**, *11*, 1–49.

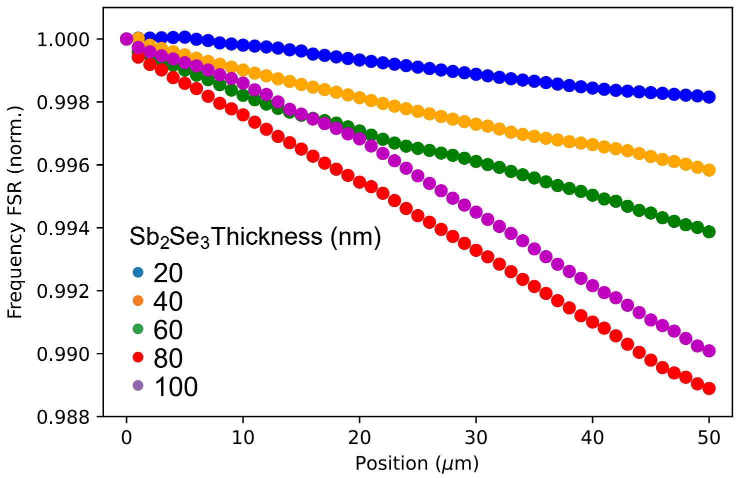


Figure 10: Fitted free spectral range normalized to initial value before switching, against write laser position along the PCM slab, for devices with different $Sb_2Se_3$ thickness of 20, 40, 60, 80, and 100 nm.


(2) Kane Yee Numerical solution of initial boundary value problems involving maxwell's equations in isotropic media. *IEEE Transactions on Antennas and Propagation* **1966**, *14*, 302–307.

(3) Yang, S.; Ma, Y.; Hochberg, M.; Baehr-Jones, T.; Novack, A.; Ding, R.; Lim, A. E.-J.; Lo, G.-Q.; Zhang, Y. Ultralow loss single layer submicron silicon waveguide crossing for SOI optical interconnect. *Optics Express, Vol. 21, Issue 24, pp. 29374-29382* **2013**, *21*, 29374–29382.

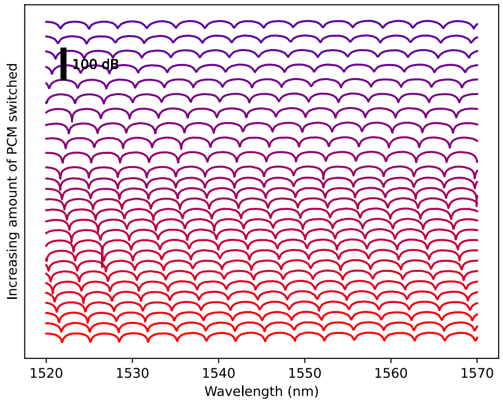


(a) 40nm deposition

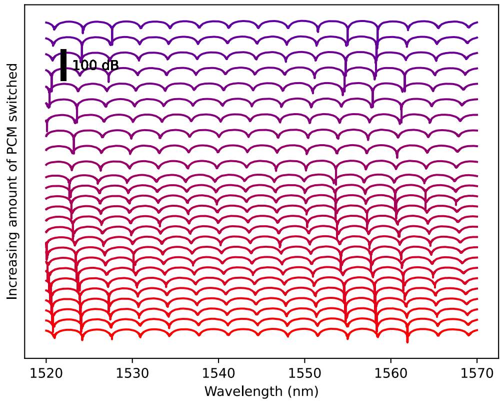


(b) 60nm deposition

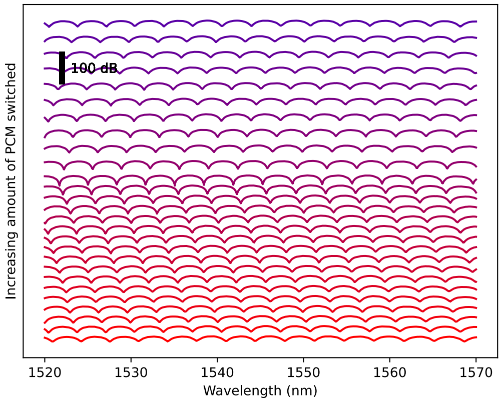


(c) 80nm deposition

Figure 11: Switching 1$\mu$m of PCM on an MZI arm and taking the spectrum after each switching performed. These Fig.s show every fifth spectrum taken as 50$\mu$m in total was amorphized and recrystallized, after an initial burn-in crystallisation.The subfigures show this process for three different deposition thicknesses and corresponding etch depths; sample a) was etched 20nm and 40nm of $Sb_2Se_3$ deposited, sample b) was etched 40nm and 60nm of $Sb_2Se_3$ deposited, and sample c) was etched 60nm and 80nm of $Sb_2Se_3$ deposited.

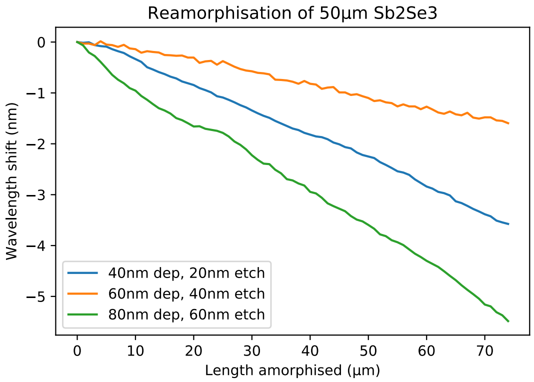


(a)

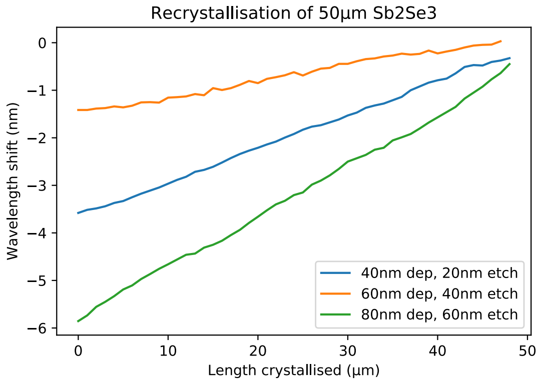


(b)

Figure 12: Wavelength shift of spectra taken after each 1$\mu$m of switching is performed. This data is taken after an initial burn-in crystallisation step is performed on the as-deposited amorphous material. 50$\mu$m are then gradually (a) reamorphized and (b) recrystallized.

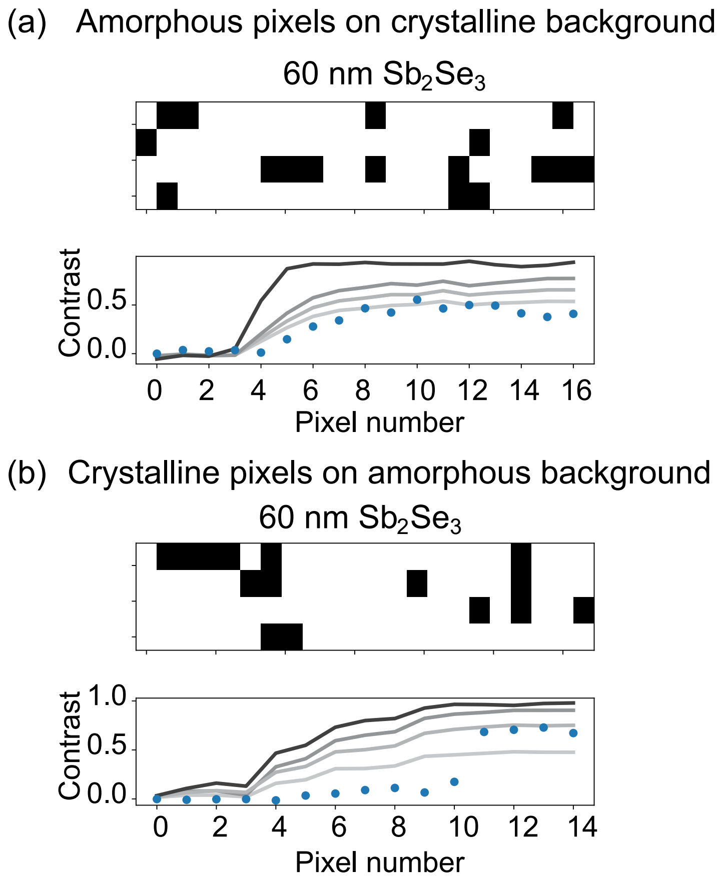


Figure 13: Switching contrast against pixel number for the digital patterns for the devices with 60 nm $Sb_2Se_3$ thickness, with simulations performed at different etch depth conditions of 0% (no etch), 25%, 50% and 100% of the $Sb_2Se_3$ layer thickness minus 20 nm, and experimental results (blue dots). Data presented for amorphous pixels on crystalline background (a) and crystalline pixels on amorphous background (b).
